# Supplementary material for: McNdroid: A Longitudinal Multimodal Benchmark for Robust Drift Detection in Android Malware
Source: arXiv:2605.06894 source file (2026-05-07)
Supplement: Supplementary file 1 [file feature-umap.tex]

% \begin{figure*}[t]
%     \centering
%     \setlength{\tabcolsep}{1.2pt}
%     \renewcommand{\arraystretch}{0.85}

%     \newcommand{\umapfig}[1]{%
%         \adjustbox{valign=m}{\includegraphics[width=0.15\textwidth]{#1}}%
%     }
%     \newcommand{\rowlabel}[1]{%
%         \adjustbox{valign=m}{%
%             \makebox[0.035\textwidth][c]{\rotatebox[origin=c]{90}{\textbf{#1}}}%
%         }%
%     }

%     \resizebox{\textwidth}{!}{%
%     \begin{tabular}{c c c c c c c}

%         & \textbf{2014} & \textbf{2016} & \textbf{2017}
%         & \textbf{2018} & \textbf{2019} & \textbf{2020} \\[-0.25em]

%         \rowlabel{Static} &
%         \umapfig{figures/data_drift/umap_pair_data_2013_vs_2014.pdf} &
%         \umapfig{figures/data_drift/umap_pair_data_2013_vs_2016.pdf} &
%         \umapfig{figures/data_drift/umap_pair_data_2013_vs_2017.pdf} &
%         \umapfig{figures/data_drift/umap_pair_data_2013_vs_2018.pdf} &
%         \umapfig{figures/data_drift/umap_pair_data_2013_vs_2019.pdf} &
%         \umapfig{figures/data_drift/umap_pair_data_2013_vs_2020.pdf}
%         \\[0.25em]

%         \rowlabel{Dynamic} &
%         \umapfig{figures/json_drift/umap_pair_json_2013_vs_2014.pdf} &
%         \umapfig{figures/json_drift/umap_pair_json_2013_vs_2016.pdf} &
%         \umapfig{figures/json_drift/umap_pair_json_2013_vs_2017.pdf} &
%         \umapfig{figures/json_drift/umap_pair_json_2013_vs_2018.pdf} &
%         \umapfig{figures/json_drift/umap_pair_json_2013_vs_2019.pdf} &
%         \umapfig{figures/json_drift/umap_pair_json_2013_vs_2020.pdf}
%         \\[0.25em]

%         \rowlabel{Graph} &
%         \umapfig{figures/gml_drift/umap_pair_gml_2013_vs_2014.pdf} &
%         \umapfig{figures/gml_drift/umap_pair_gml_2013_vs_2016.pdf} &
%         \umapfig{figures/gml_drift/umap_pair_gml_2013_vs_2017.pdf} &
%         \umapfig{figures/gml_drift/umap_pair_gml_2013_vs_2018.pdf} &
%         \umapfig{figures/gml_drift/umap_pair_gml_2013_vs_2019.pdf} &
%         \umapfig{figures/gml_drift/umap_pair_gml_2013_vs_2020.pdf}
%         \\[0.35em]

%         \multicolumn{7}{c}{%
%         \begin{tabular}{c c c c c c}
%             & \textbf{2021} & \textbf{2022} & \textbf{2023}
%             & \textbf{2024} & \textbf{2025} \\[-0.25em]

%             \rowlabel{Static} &
%             \umapfig{figures/data_drift/umap_pair_data_2013_vs_2021.pdf} &
%             \umapfig{figures/data_drift/umap_pair_data_2013_vs_2022.pdf} &
%             \umapfig{figures/data_drift/umap_pair_data_2013_vs_2023.pdf} &
%             \umapfig{figures/data_drift/umap_pair_data_2013_vs_2024.pdf} &
%             \umapfig{figures/data_drift/umap_pair_data_2013_vs_2025.pdf}
%             \\[0.25em]

%             \rowlabel{Dynamic} &
%             \umapfig{figures/json_drift/umap_pair_json_2013_vs_2021.pdf} &
%             \umapfig{figures/json_drift/umap_pair_json_2013_vs_2022.pdf} &
%             \umapfig{figures/json_drift/umap_pair_json_2013_vs_2023.pdf} &
%             \umapfig{figures/json_drift/umap_pair_json_2013_vs_2024.pdf} &
%             \umapfig{figures/json_drift/umap_pair_json_2013_vs_2025.pdf}
%             \\[0.25em]

%             \rowlabel{Graph} &
%             \umapfig{figures/gml_drift/umap_pair_gml_2013_vs_2021.pdf} &
%             \umapfig{figures/gml_drift/umap_pair_gml_2013_vs_2022.pdf} &
%             \umapfig{figures/gml_drift/umap_pair_gml_2013_vs_2023.pdf} &
%             \umapfig{figures/gml_drift/umap_pair_gml_2013_vs_2024.pdf} &
%             \umapfig{figures/gml_drift/umap_pair_gml_2013_vs_2025.pdf}
%         \end{tabular}%
%         }

%     \end{tabular}%
%     }

%     \vspace{-0.6em}
%     \caption{UMAP visualization of temporal representation drift across modalities. Each column compares the 2013 training distribution against a later test year, showing how modality-specific feature spaces evolve under increasing temporal shift.}
%     \label{fig:umap_drift_all_years}
% \end{figure*}
